# Supplementary material for: Simulating Before Planning: Constructing Intrinsic User World Model for User-Tailored Dialogue Policy Planning
Source: arXiv:2504.13643 source file (2025-04-18)
Supplement: Supplementary file 1 [file 6-appendix.tex]

\appendix
\section{Proofs for Optimization Objectives}
